# Supplementary material for: First-principles calculation of the entropy of liquids with a case study on sodium
Source: arXiv:2411.10930 source file (2024-11-17)
Supplement: Supplementary file 1 [file Supplement.pdf]

# Supplemental Materials to "First-principles calculation of entropy of a liquid: with a case study on Na"

Koun Shirai[1,2], Hiroyoshi Momida[3], Kazunori Sato[4], and Sangil Hyun[5]
[1] SANKEN, Osaka University
8-1 Mihogaoka, Ibaraki, Osaka 567-0047, Japan
[2]Vietnam Japan University, VNU, Hanoi,
Luu Huu Phuoc Road, My Dinh 1 Ward,
Nam Tu Liem District, Hanoi, Vietnam
[3]Advanced Materials Laboratory, Sumitomo Electric Industries, Ltd.
1-1-1 Koyakita, Itami, Hyogo 664-0016, Japan
[4]Graduate School of Engineering, Osaka University
2-1 Yamadaoka, Suita, Osaka 565-0871, Japan
[5]Korea Institute of Ceramic Engineering and Technology
101 Soho-ro, Jinju-si, Gyeongsangnam-do, 52851, Korea

November 17, 2024

# 1 Convergence

The convergence for the melting temperature $T_m$ against various parameters in FPMD simulations is tested. In Fig. 1, the structural energy, $E_{\rm st}$, and diffusion constant, $D$, are plotted as functions of $T$ for various parameters. The most significant parameter is the cell size. Cell sizes of $N$ =16 and 128 atoms were examined. When different sizes of supercells are compared, the equivalent $k$ meshes should be use. Thus, the data obtained by a $2^3$ $k$-mesh (denoted by nkdiv=2) for the 16-atom cell (crosses in the figure) should be compared with the data obtained by a 1 $k$-mesh (denoted by nkdiv=1) for the 128-atom (red circles). Clearly, the $T_m$ value is lowered from 600 to 460 K by increasing the cell size from 16 to 128. But the calculated value is still too high compared to the experimental value 371 K.

For metallic systems, the $k$ mesh can affect the total energy calculation largely. Hence, the dependence of the $k$ mesh was also examined for the 128-atom cell. However, there was only a marginal change in $T_m$ between 1 (red circles) and $2^3$ (blue circles) meshes, as shown in this figure. After this calculation, we fixed the cell size $N$ =128, and $2^3$ $k$-mesh.

Up to this, the electron occupancies, $f_e(\epsilon)$, have been fixed as the ground-state occupancies. Technically, in the Phase/0 code, a slight smearing $\sigma$ is applied to $f_e(\epsilon)$. However, this $\sigma$ is fixed and is independent of temperature. In real electron systems, $f_e(\epsilon)$ obeys the Fermi-Dirac distribution, $f_e(\epsilon) = 1/(e^{\beta(\epsilon-\mu_e)}+1)$, where $\mu_e$ is the electron chemical potential and $\beta = 1/k_{\rm B}T$. The Fermi-Dirac distribution was applied to the MD simulation, which is indicated by the open triangles. This brings a slight decrease in $E_{\rm st}$ in the liquid phase, but no change in $T_m$ and $D$.

In all the calculations up to here, the volume of the unit cell was fixed at the volume of the crystal Na, namely, $V_{(s)}$ = 22.69 cm$^3$/mol. When it melts, the volume expands by 9.4 %. The MD simulations were examined with $V_{(l)}$ = 24.84 cm$^3$/mol, which are indicated by black diamonds. Now, we observe that the calculated value is just the experimental value 371 K.

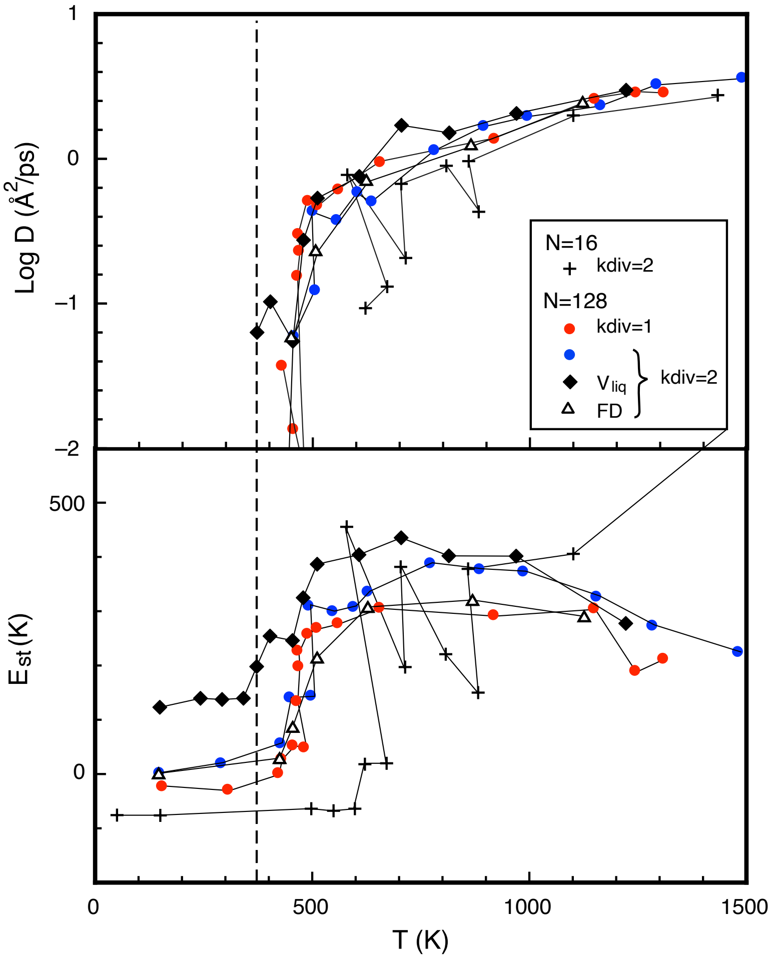


Figure 1: The diffusion coefficient, $D$, and structural energy, $E_{\rm st}$, of Na calculated by NC+GGA. Cell sizes are $N = 16$ and 128. The $k$ meshes are $2^3$ for $N = 16$, whereas are 1 (red circles) and $2^3$ (blue circles) for $N = 128$. $E_{\rm cut} = 245$ eV. For each $N$, the energy origin was set to the ground state energy for that cell. FD (open triangles) indicates the results when the Fermi-Dirac distribution is adapted. $\rm V_{liq}$ (black diamonds) indicates the results when the volume is expanded to be that of the liquid. The experimental value for $T_m$ is indicated by the dashed line.

## 2 Phonon spectrum

Evolution of phonon spectra of Na when the solid Na is heated to melt is shown in Fig. 2. These spectra were obtained from MD simulations with total simulation time, $t_{\rm sm} = 2.4$ ps, which limits the frequency resolution $\Delta\omega = 13.8\ {\rm cm}^{-1}$. As shown here, the phonon spectra of the liquid is basically a broadened form of that of the crystal. Note that non-zero components appear at $\omega = 0$ on melting.

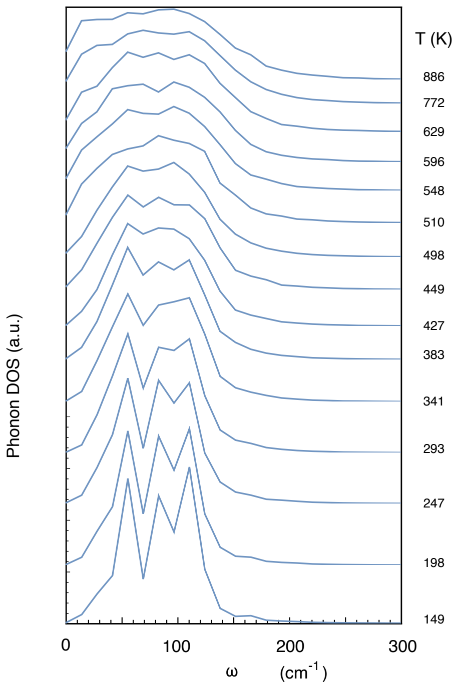


Figure 2: Temperature dependence of the phonon spectra of Na.
